# Supplementary material for: LiVOS: Light Video Object Segmentation with Gated Linear Matching
Source: arXiv:2411.02818 source file (2024-11-05)
Supplement: Supplementary file 1 [file X_suppl.tex]

\clearpage
\setcounter{page}{1}
\maketitlesupplementary

% \section{Rationale}
% \label{sec:rationale}
% % 
% Having the supplementary compiled together with the main paper means that:
% % 
% \begin{itemize}
% \item The supplementary can back-reference sections of the main paper, for example, we can refer to \cref{sec:intro};
% \item The main paper can forward reference sub-sections within the supplementary explicitly (e.g. referring to a particular experiment); 
% \item When submitted to arXiv, the supplementary will already included at the end of the paper.
% \end{itemize}
% % 
% To split the supplementary pages from the main paper, you can use \href{https://support.apple.com/en-ca/guide/preview/prvw11793/mac#:~:text=Delete%20a%20page%20from%20a,or%20choose%20Edit%20%3E%20Delete).}{Preview (on macOS)}, \href{https://www.adobe.com/acrobat/how-to/delete-pages-from-pdf.html#:~:text=Choose%20%E2%80%9CTools%E2%80%9D%20%3E%20%E2%80%9COrganize,or%20pages%20from%20the%20file.}{Adobe Acrobat} (on all OSs), as well as \href{https://superuser.com/questions/517986/is-it-possible-to-delete-some-pages-of-a-pdf-document}{command line tools}.

% \section{Related Work}

% \paragraph{Interactive VOS.}
% Semi-supervised VOS can be seen as a special form of interactive VOS.

\section{Baselines}

\noindent \textbf{AOT}~\cite{yang2021associating} and \textbf{DeAOT}~\cite{yang2022decoupling} are two consecutive approaches to improve the efficiency of VOS with multiple objects. Following Cutie~\cite{cheng2024putting}, we use the model variants with a ResNet-50 backbone as baselines. 

\noindent \textbf{CFBI}~\cite{yang2020collaborative} and \textbf{CFBI+}~\cite{yang2021collaborative} propose a collaborate VOS approach that integrates both foreground and background information into embedding learning. As they only use two memory frames, we classify them as non-STM methods with less strict criteria. Both models use RestNet-101 as the backbone, and we adopt them as our baselines.

\noindent \textbf{DEVA}~\cite{cheng2023tracking} decouples task-specific image-level segmentation and mask propagation for universal video segmentation. We use as the model trained solely on YouTube-VOS~\cite{xu2018youtube} and DAVIS 2017~\cite{perazzi2016benchmark} as the baseline.

\noindent \textbf{SwiftNet}~\cite{wang2021swiftnet} balances accuracy and speed by compressing spatiotemporal redundancy in matching-based VOS with a pixel-adaptive memory. We use the model variant with a ResNet-50 backbone as the baseline.

\noindent \textbf{MobileVOS}~\cite{miles2023mobilevos} distills knowledge from a teacher model utilizing large backbone and infinite memory. We use the best-performing model variant with a ResNet-18 backbone as the baseline.

\section{Implementation Details}

\paragraph{Sensory Memory.} We adopt sensory memory~\cite{cheng2022xmem} to maintain low-level information such as object location. A sensory memory stores a hidden state $\mathbf{H}_{t+1} \in \mathbb{R}^{HW\times C_h}$, initialized as a zero vector, and propagated by a Gated Recurrent Unit (GRU)~\cite{cho2014properties}. The hidden state $\mathbf{H}_{t+1}$ is updated every frame using multi-scale features of the mask encoder and decoder, and is added to the value readout $\mathbf{V}_{t+1}$. We set the sensory feature dimension $C_h$ to 256.

\paragraph{Object Memory.} We enrich the value readout $V_{t+1}$ for the query frame with object-level semantics using an object transformer~\cite{cheng2024putting}. The object transformer takes the initial value readout $\mathbf{V}_{t+1} \in \mathbb{R}^{HW\times C_v\times N}$, a set of $M$ end-to-end trained object queries $\mathbf{Q} \in \mathbb{R}^{M\times C}$ and object memory $\mathbf{O} \in \mathbb{R}^{N\times C}$, and integrates them with $L$ transformer blocks. We set the number of object transformer blocks $L$ to 3 and the number of object queries $M$ to 16. 

\paragraph{Training.} We do not use static images for pretraining as we observe no significant improvement.

\paragraph{Inference.}

Evaluation on multiple objects. and evaluation for high-resolution videos. This section will introduce experimental details for evaluation on high-resolution videos.

\section{Qualitative Results}
\label{sec:qualitative_results}

We show some qualitative results here.

\section{Computational Analysis}

\begin{figure}[ht]
    \centering
    \includegraphics[width=0.85\linewidth]{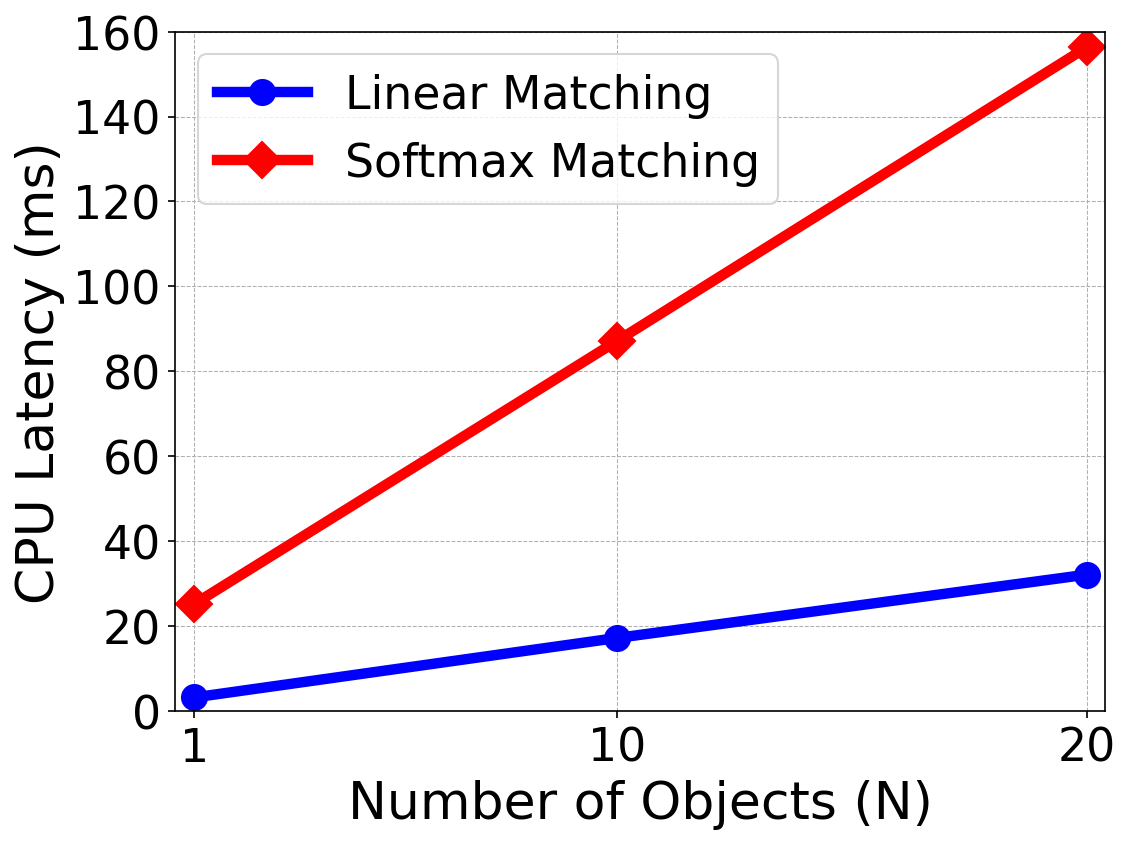}    
    \caption{\emph{CPU latency comparison between softmax matching and linear matching}. Linear attention scales linearly with input resolution and object number, while softmax attention scales quadratically with input resolution. Latency is measured on an Intel Core-i7 (2.80GHz) CPU with PyTorch 2.0, batch size 1, and fp32.}
    \label{fig:cpu_latency_n}
\end{figure}

% \section{Discussions}
% \label{sec:discussions}

% Our method may slow down when tracking a large number of objects (e.g., over 1,000) due to its linear complexity with respect to the number of objects. In such case, the identification mechanism in AOT~\cite{yang2021associating} is a promising solution. Additionally, our method may struggle in scenarios involving similar objects in close proximity, fast movement, or occlusion. We believe large-scale training could mitigate these issues to some extend.
